# Supplementary material for: YOPO-Nav: Visual Navigation using 3DGS Graphs from One-Pass Videos
Source: arXiv:2512.09903 source file (2025-12-10)
Supplement: Supplementary file 1 [file X_suppl.tex]

\clearpage
\setcounter{page}{1}
\maketitlesupplementary

\setcounter{section}{0}

\section{Overview}
\label{sec:suppl_overview}

The supplementary material includes this file as well as several videos that could not be embedded in this PDF. We organized the supplementary material organized into seven main sections. In Section \ref{section:supp_dataset_videos}, we describe examples of egocentric videos from the dataset, which we include in the files of this submission. In Section \ref{section:supp_ground_plane}, we showcase the ground plane masks produced by SAM-2.1 in the simulated environment across several trajectory videos. In Section \ref{section:supp_3dgs_actions}, we compare the ground truth actions to the actions produced by the action generation module across several trajectory videos. In Section \ref{section:supp_anysplat_metrics}, we report the metrics of 3DGS models produced by AnySplat \cite{jiang2025anysplat}. In Section \ref{section:supp_path_planning}, we describe the simple path planning algorithm in more detail and provide a brief analysis on its efficacy. In Section \ref{section:supp_yoponav_recordings}, we present a screen recording of the YOPO-Nav GUI, captured while running an experiment detailed in Subsection \ref{subsec:human_intervention_exprs}. This recording is included. In Section \ref{section:supp_yoponav_sota_recordings}, we show some example egocentric videos from the experiments that were ran on ViNT/NoMaD, in Subsection \ref{subsec:sota_comparisons} and discuss the results. These videos are included. 

We also include the Egocampus dataset paper \cite{Anonymous2025}, a concurrent submission under review for CVPR 2026, in our supplementary material. This is labeled as \texttt{ego\_campus.pdf}. We also included statistics (e.g. number of actions, elapsed time, and distance traveled) for each trajectory in YOPO-Campus, which is labeled as \texttt{yopo\_campus\_stats.txt}. In the file, each trajectory is assigned a numerical label, followed by an underscore and a second numerical label indicating its direction.

\section{Dataset Egocentric Videos}
\label{section:supp_dataset_videos}

Egocentric videos from the YOPO-Campus dataset, introduced in Subsection \ref{subsec:yopo-campus}, are included in the supplementary material to illustrate representative examples of the trajectory videos. Portions from two trajectories were carefully selected to avoid inclusion of identifiable information. The trajectories consist of a simple straight line along a sidewalk and a curved sidewalk that transitions into a road. Frames in which the Jackal robot rotated in-place were removed out of precaution. As discussed, this occurs at points where the sidewalk diverges into multiple paths. The corresponding files are labeled as \texttt{dataset\_examples/straight\_line\_path.mp4} and \texttt{dataset\_examples/curvy\_path.mp4}. These two example trajectories will be used in Sections \ref{section:supp_3dgs_actions} and \ref{section:supp_anysplat_metrics}.

\section{Ground Plane Segmentation Results}
\label{section:supp_ground_plane}

\begin{figure*}
\centering
\includegraphics[width=\textwidth, height=0.3\textheight]{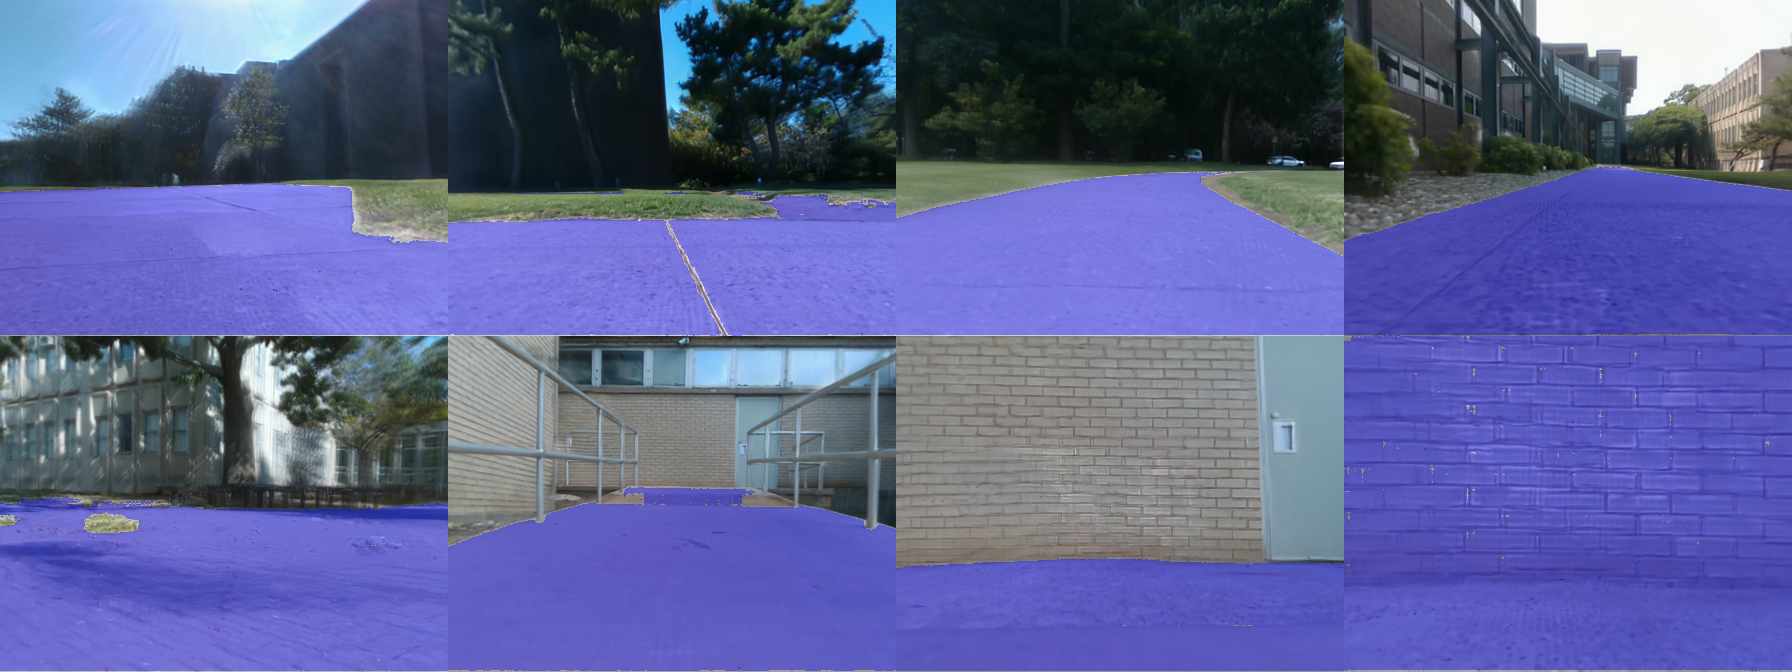}
\caption{
\textbf{SAM-2.1 Ground Plane Masks} Ground plane masks from eight images across five unique trajectories are shown. The mask is superimposed on the original images as a semi‑transparent blue overlay. Overall, with a single point click, SAM‑2 estimates the ground plane, which we define as the sidewalk, road, or brick pavement that forms the trajectory, reliably, with only a few exceptions: obstructing surfaces, such as leaves on top of the ground, cases where the Jackal robot is too close to a wall, or off‑trajectory regions containing similarly colored surfaces, such as sand right next to the sidewalk.}
\label{fig:sam2_ground_plane_masks}
\end{figure*}

As previously explained in the navigation paragraph of Subsection \ref{subsec:yoponav}, RGB images at each known pose in the 3DGS models are rendered and point clicks, positioned at the bottom 90\% of the image height and centered along the image width, are provided to the multi-mask version of SAM-2.1 to isolate the ground planes. It is assumed that, across each image, the ground planes will exist in this region—and it should exist based on our data collection procedure. The largest mask is always used to ensure the as much of the ground plane is segmented as possible.

In Fig.~\ref{fig:sam2_ground_plane_masks} we show eight example images across five unique trajectories. We define the ground plane as sidewalk, road, or brick pavement that forms the trajectory the Jackal robot follows. The first two images on the top (left to right) are from the same trajectory and, in the first image, the ground plane is estimated rather well, but in the second image, an extraneous region of sand is included, mainly because the surface is right next to the sidewalk and is a similar color. The last two images on the top are from two separate trajectories and the segmentation result is sufficient. The first image on the bottom contains a brick pavement surface, instead of a sidewalk, and segmentation is sufficient. Leaves on the ground obstructed the surface in two spots and thus affected the segmentation result but this is largely negligible. The ground plane is estimated from top 30\% of pixels closest to the camera. The last three images come from the same trajectory. The first shows a slope, where segmentation is largely sufficient, with some exceptions at the top. Once again, this area would likely not be used for ground plane estimation. The next image depicts the robot near a wall, which produces an acceptable segmentation of the ground. In the final image, where the robot is very close to the wall, segmentation fails catastrophically, covering the entire image. This is the only severe failure case observed. Since minimizing inference time was a priority, we used the base SAM-2.1 model with a point click; at the cost of inference time, the results could be improved using a version of SAM-2.1 that fuses segmentation with language-understanding, which would largely fix the observed issues.

\section{Action Generation Module Results}
\label{section:supp_3dgs_actions}

We computed the error between the actions in the 3DGS simulation environment and the ground truth actions using the two trajectories that we included in the supplementary material and discussed in \ref{section:supp_dataset_videos}. That is, we started from the first frame in the video and had the agent in the 3DGS simulation navigate to the last frame in the video. These videos illustrate two cases: a straight trajectory and a curvy trajectory. The rotation and translation errors were calculated calculated individually.

In the simulation environment, each video frame is traversed by applying a sequence of rotations and translations, derived from estimating the pose change required to move from the current frame to the next. From this pose change, the rotation and translation components are extracted. For the rotation component we take only take the yaw, and we do not use the rotations from the three‑action pipeline discussed previously in the navigation paragraph of Subsection \ref{subsec:yoponav}. We use the yaw directly. The translation component is converted to metric units using the scale factor derived from SAM‑2.1 ground plane estimation. For the ground truth, the change in compass direction (from the Pixel 3a) between consecutive frames is used, rather than the $15^\circ$ approximation from the ROS Angular Twist messages that were used during data collection (discussed in Section \ref{subsec:yopo-campus}. The translation cannot reliably be derived from the change in GPS coordinates between consecutive frames due to drift. Therefore, the translation is computed by by mapping the \SI{1.0}{\meter\per\second} velocity from the linear ROS twist messages that we used during data collection to \SI{0.25}{\meter}.

Following this setup, we report the mean and standard deviation of rotation and translation errors between corresponding simulation and ground-truth points along each trajectory, and additionally include the Fréchet distance as a global measure of trajectory similarity. The results are shown in table \ref{tab:path-errors}. Fréchet distance captures the maximum deviation under optimal traversal, reflecting the worst‑case discrepancy between simulation trajectory and ground-truth trajectory. The Straight-Line trajectory was observed to have a much larger Fréchet distance compared to the Curvy trajectory, while the Curvy trajectory was observed to have larger rotation errors. Translation errors were roughly the same. Since the curvy trajectory contains bends, rotation errors are naturally larger. However, these bends limit sustained lateral drift, so the worst‑case separation is smaller, yielding a lower Fréchet distance than the Straight‑Line trajectory.

Errors accumulated from a combination of two factors: the scale factor used to convert the simulated translations to metric units and the estimated camera poses from AnySplat \cite{jiang2025anysplat}. Most likely, the estimated camera poses are within the margin of error reported by VGGT \cite{wang2025vggt}, which AnySplat depends upon. It was observed that AnySplat had extraneous translations when the Jackal robot was rotating in place, so camera pose errors on the centimeter scale are possible. Additionally, in some cases, the camera pose estimations may drift from their location in the real-world, and then instruct it to go somewhere else then what is intended. Since the ground truth translations are approximations, it is also possible that the forward and backward actions are closer to \SI{0.20}{\meter}, than \SI{0.25}{\meter}. This may be the case because the Straight-Line trajectory reported a mean translation error of \(\SI{0.2049}{m} \pm \SI{0.053}{m}\), while the Curvy trajectory reported a mean translation error of \(\SI{0.1968}{m} \pm \SI{0.047}{m}\). The ground-truth translations will also have real-world inconsistencies that would not be accounted for with the \SI{0.25}{\meter} estimation.

\begin{table}
  \centering
  \scriptsize
  \setlength{\tabcolsep}{3pt}
  \scalebox{0.95}{
    \begin{tabular}{@{}lccc@{}}
      \toprule
      Path & Rotation Error (°) ↓ & Translation Error (m) ↓ & Fréchet Distance (m) ↓ \\
      \midrule
      Straight-Line & $1.21 \pm 2.11$ & $0.07 \pm 0.04$ & 13.3 \\
      Curvy         & $2.76 \pm 4.70$ & $0.05 \pm 0.03$ & 5.8 \\
      \bottomrule
    \end{tabular}
  }
  \caption{Comparison of trajectory errors across straight-line and curvy paths. Fréchet distance is reported for each trajectory along with the mean and standard deviation rotation and translation errors. The Straight-Line trajectory is \SI{30}{\meter} long and the Curvy trajectory is \SI{55}{\meter} long. The mean translations errors are roughly the same on both trajectories; however the rotation error on the Curvy trajectory is rougher twice as large. The Fréchet distance is roughly twice as large on the Straight-Line trajectory compared to the Curvy trajectory.}
  \label{tab:path-errors}
\end{table}

\section{AnySplat Results}
\label{section:supp_anysplat_metrics}

As discussed in the 3DGS paragraph of Section \ref{subsec:yoponav}, AnySplat produced the best results compared to alternative pose-free Gaussian splatting methods. That is, it produced the least sparse representation with the most accurate camera poses. Following the two trajectories that were detailed in Section \ref{section:supp_dataset_videos}, we present metrics for the 3DGS models that make up each trajectory in table \ref{tab:path-quality}. The Curvy Trajectory consists of 195 frames so there are 4 3DGS models while the Straight-Line Trajectory consists of 143 frames so there are 3 3DGS. This follows the procedure outlined in the Implementation Details paragraph in Subsection \ref{subsec:sota_comparisons}, where each 3DGS is constrained to at most 55 images. The reconstruction quality is acceptable enough to perform PnP-RANSAC between the Jackal robot's camera feed and the 3DGS models. Videos of an agent navigating in these 3DGS for the two trajectories are included with the supplementary material. See \texttt{simulation\_examples/curvy\_path.mp4} and \texttt{simulation\_examples/straight\_line\_path.mp4} for more details.

\begin{table}[!b]
  \centering
  \scriptsize
  \setlength{\tabcolsep}{3pt}
  \scalebox{1.05}{
    \begin{tabular}{@{}lccc@{}}
      \toprule
      Trajectory & PSNR (dB) ↑ & SSIM ↑ & LPIPS ↓ \\
      \midrule
      Curvy – 3DGS 1 & $21.57 \pm 2.22$ & $0.572 \pm 0.081$ & $0.341 \pm 0.049$ \\
      Curvy – 3DGS 2 & $19.87 \pm 2.91$ & $0.543 \pm 0.102$ & $0.366 \pm 0.066$ \\
      Curvy – 3DGS 3 & $19.06 \pm 1.62$ & $0.491 \pm 0.061$ & $0.360 \pm 0.041$ \\
      Curvy – 3DGS 4 & $18.60 \pm 1.56$ & $0.355 \pm 0.079$ & $0.396 \pm 0.051$ \\
      \midrule
      Straight-Line – 3DGS 1 & $22.03 \pm 1.67$ & $0.627 \pm 0.040$ & $0.362 \pm 0.032$ \\
      Straight-Line – 3DGS 2 & $23.07 \pm 1.79$ & $0.591 \pm 0.068$ & $0.320 \pm 0.042$ \\
      Straight-Line – 3DGS 3 & $19.39 \pm 1.26$ & $0.463 \pm 0.057$ & $0.412 \pm 0.025$ \\
      \bottomrule
    \end{tabular}
  }
  \caption{Comparison of PSNR, SSIM, and LPIPS across Curvy and Straight-Line trajectories. Each row corresponds to one 3D Gaussian Splatting (3DGS) component of a trajectory.}
  \label{tab:path-quality}
\end{table}

\section{Simple Path Planning Results}
\label{section:supp_path_planning}

Path planning is performed by calculating the minimal frame sequence between a starting image—which was automatically determined by matching the current observation from the Jackal robot's camera to the closest image in the FAISS index—and a goal image that was manually selected in the GUI. The graph network has a node for each image and an edges that correspond to nearby images from other trajectories, if they exist. As discussed in the 3DGS paragraph of Subsection \ref{subsec:yoponav}, this approach is meant to be simple and lightweight, as it relies on the existing architecture of YOPO-Nav: YOPO-Loc and point correspondences from XFeat \cite{potje2024xfeat}. It works best when two trajectories share segments that align in the same real‑world location, rather than merely overlapping visually, since no depth calculations are utilized. In some instances, when visual overlap occurs, the jump from one trajectory to another skips a couple of meters, at most, in real-world distance that requires a human to correct. In most other cases, the path planning algorithm works sufficiently, but due to the nature of how YOPO-Campus was collected, the algorithm tends to jump from one trajectory to another at the instances where the Jackal robot was rotated in place. This means that, because rotations were not consistently executed at the same locations across nearby trajectories, the path planning algorithm occasionally requires the Jackal robot to advance to a point where an in‑place rotation occurred on one trajectory, switch to the other trajectory, and then backtrack along the new trajectory to reach the goal.

Path planning was briefly tested in Subsection \ref{subsec:human_intervention_exprs}, specifically the Combined Trajectory in table \ref{tab:yopo-interventions}. This path had real-world overlap, rather than nearby visual overlap, and worked extremely well, but due to having identifying information, this path could not be included in the supplementary material. We included the case where two trajectories were nearby and there was a several-meter jump from one trajectory to another. This file is labeled as \texttt{planning\_examples/jump.mp4}. We also included the case where two trajectories were nearby but there was only a slight jump from one trajectory to another. This file is labeled as \texttt{planning\_examples/slight\_jump.mp4}.

\section{Recording from YOPO-Nav Experiments}
\label{section:supp_yoponav_recordings}

We included a portion from a screen recording of the YOPO-Campus GUI, which was captured when running the Straight Trajectory in table \ref{tab:yopo-interventions}. This is labeled as \texttt{gui\_recording/straight\_trajectory.mp4}. The full recording of this experiment or portions from other experiments could not be included because of identification purposes. This trajectory is similar to the Straight-Line trajectory shown in the previous sections of the supplementary material. Five minutes of the total experiment are shown, starting at roughly the beginning, of the YOPO-Nav following the recorded trajectory autonomously. That is, no human intervention was required. For 15 seconds in the video, the Jackal camera feed is blurred because an individual walks by in the scene. Overall, YOPO-Nav matches the trajectory quite accurately and is able to successfully navigate \SI{45}{\meter} autonomously in this simple scenario.

The entirely of YOPO-Campus can be evaluated in this video—the 3DGS simulation environment, YOPO-Loc, Pose Estimation Module, and Action Generation Module—that we outlined in fig. \ref{fig:yoponav}. In the top left of the GUI, the Jackal camera feed is shown, in the bottom left the closest match in YOPO-Campus is shown, and the bottom right shows the simulation environment. Though this task is simple, and the algorithm performs adequately, the video provides one definitive conclusion: YOPO-Loc, the VPR model, is the main bottleneck of YOPO-Campus. This is mainly because of its precision and its variable resistance to season and lighting changes, if it dominates the scene. YOPO-Loc was trained to achieve \SI{0.50}{\meter} localization accuracy, and although for the most part it works, in the video it can be seen that the closest matched frame sometimes jumps around quite a bit (moves forward and back in time). Additionally, there are some instances where it matches to a completely different, erroneous trajectory. This occurs more commonly in areas where there are a lot of surrounding trajectories. In YOPO-Nav the VPR model is queried during the initialization localization, that is when a path is planned, and after a human is done intervening. The initialization localization was qualitatively a minor issue, since the algorithm is able to latch back onto the path if the starting point is not fully correct, but the human interventions were a problem. On occasion, YOPO-Loc would localize to a point that was ahead or behind, and sometimes it would get stuck and the human intervention would loop. This occurred most commonly in the Construction Area experiment that was conducted in table \ref{tab:yopo-interventions}. For improved accuracy, YOPO-Loc would have to be trained on large datasets or combined with object-detection and other tools.

Besides the YOPO-Loc failures that were somewhat shown in the example video and discussed in Subsection \ref{subsec:human_intervention_exprs}, the other main failure was PnP RANSAC. Though not observed in this video, sometimes the agent would localize completely off of the 3DGS, so much so that it was visually apparent. When this happened, the agent generate an action that consisted of an extremely large translation, which would be ignored by the Action Generation Module on principle. In these cases, the human would have to intervene and nudge the Jackal robot slightly, and this usually fixed the issue.

\section{SOTA Recordings}
\label{section:supp_yoponav_sota_recordings}
\textbf{Success and Failure Cases}

We tested ViNT \cite{shah2023vint} and NoMad \cite{sridhar2024nomad} in the YOPO-Campus environment as discussed in Section \ref{subsec:sota_comparisons}. These visual navigation models exhibited similar success and failure cases across each set of trials. Trials on exploration paths with straight trajectories had higher success rates, while paths with turns exhibited several different failure cases. A sample success case can be found in \texttt{sota/success.mp4}, with its corresponding ground truth exploration video found in \texttt{sota/success\_gt.mp4}. Notice how the exploration path trajectory is relatively straight, and the main action is forward. Sample failure cases can be found in \texttt{sota/failures.mp4}, with its corresponding ground truth exploration video found in \texttt{sota/failures\_gt.mp4}. These trials showcase three main failure cases: the model not recognizing the goal image, the model colliding with an object, and the model straying away from the exploration path. In the first trial, the algorithm takes the correct set of actions to reach the goal image at 0:08, but does not recognize that it has reached the goal. The model then takes erroneous actions, leading it away from the exploration video. In the second trial, the model immediately turns right, and collides with a wall at 0:13. In the third trial, at 0:15, the model turns right and immediately leaves the exploration path. These trials highlight the potential pitfalls of end-to-end transformer models for visual navigation. Failure cases for these methods lack interpretability as to why they are taking a specific action, and what in the scene is causing them to exhibit this behavior. This contrasts with the YOPO-Nav approach, which uses camera pose to generate actions that align with the exploration video.

%\href{https://www.adobe.com/acrobat/how-to/delete-pages-from-pdf.html#:~:text=Choose%20%E2%80%9CTools%E2%80%9D%20%3E%20%E2%80%9COrganize,or%20pages%20from%20the%20file.}{Adobe Acrobat} (on all OSs), as well as \href{https://superuser.com/questions/517986/is-it-possible-to-delete-some-pages-of-a-pdf-document}{command line tools}.
